# Supplementary material for: Design of Transit-Centric Multimodal Urban Mobility System with Autonomous Mobility-on-Demand
Source: arXiv:2404.05885 source file (2024-04-08)
Supplement: Supplementary file 1 [file appendix.tex]

\appendix
